# Supplementary material for: Electrically-Reconfigurable Passive and Active Circuits in a Single Plasmonic Architecture
Source: arXiv:2011.05812 source file (2020-11-11)
Supplement: Supplementary file 1 [file supplementary_material.pdf]

# Supplementary Material for "Monolithic Plasmonic Waveguide Architecture for Passive and Active Optical Circuits"

Charles Chih-Chin Lin, Pohan Chang, Yiwen Su, and Amr S Helmy
*Department of Electrical and Computer Engineering, University of Toronto, Ontario, Canada*

## Contents

S1 Design of Coupled Hybrid Plasmonic Waveguide (CHPW) 3

S2 CHPW Modulator utilizing epsilon-near-zero effect 7

S3 CHPW-Si nanowire coupler 8

S4 CHPW Micro-ring Characteristics 11

S5 CHPW Micro-ring Characterization 12

S6 RC Bandwidth of CHPW Photodetectors 13

S7 Comparison of Experimental Plasmonic Photodetectors based on internal photoemission (IPE) 14

S8 Characterization of CHPW modulators 15

S9 RC Bandwidth of CHPW Modulators 17

S10 Comparison of Experimental ITO-based Plasmonic Modulators 18

S11 Simulated Eye Diagrams 19

References 20

## S1 Design of Coupled Hybrid Plasmonic Waveguide (CHPW)

Despite the potential for denser device integration, practical implementation of plasmonic components is impeded by the inherent modal loss associated with metal absorption [1]. As plasmonic mode volume reduces, energy will become increasingly stored in the form of carrier kinetic energy and Ohmic loss due to the metal becomes increasingly severe, especially when high-permittivity dielectric materials such as Si are involved. In order for the light-matter-interaction (LMI) afforded by plasmonic waveguides to be more effectively utilized, the propagation loss needs to be reduced without sacrificing modal confinement. Although coupled-mode plasmonic structures have demonstrated effective alleviation of the loss-confinement trade-off, stringent structural, material, and modal symmetry requirements must be enforced for such reduction to prevail [2–4]. This not only limits the material platforms that can be used, but are also easily compromised during practical implementations due to unavoidable fabrication tolerances.

The coupled hybrid plasmonic waveguide (CHPW) as shown in Fig. 1 can alleviate the loss-confinement trade-off [5]. CHPW supports supermodes formed by a superposition of hybrid plasmonic waveguide (HPW) mode with surface plasmon polariton (SPP) mode coupled through a thin metal film. The combination of dissimilar modes in one structure suggests LMI on two types of plasmonic interfaces - metal with high-index dielectric and metal with low-index dielectric. This allows one waveguide to support multiple applications. The former concentrates the field closer to the metal-dielectric interface to facilitate mechanisms such as internal photoemission. The latter confine the modal energy within the dielectric layer to enable stronger linear and nonlinear processes.

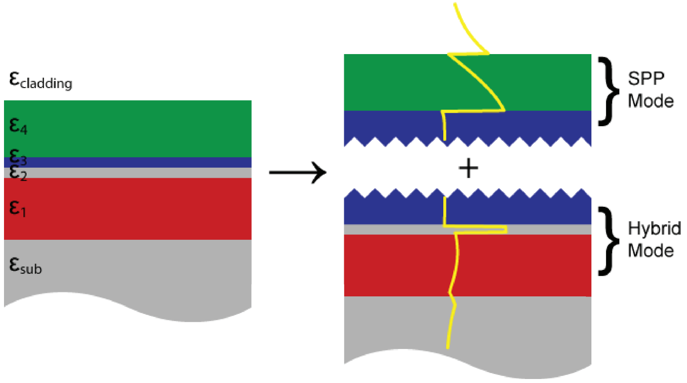


FIG. 1: CHPW is highly asymmetrical and supports supermodes that are formed by the superposition of the HPW and SPP modes coupled through a thin metal film. The asymmetry comes from material permittivity differences as well as the different constituent modal distribution and dispersion characteristics. $\epsilon_1$: high-index dielectric, $\epsilon_2$: low-index dielectric, $\epsilon_2$: metal, $\epsilon_4$: high-index dielectric.

In Fig. 2, the properties of modes guided by the CHPW structure are plotted. The dimensions on the HPW side is kept constant while thickness of the Si on the SPP side ($t_{\varepsilon 4}$) is varied. The coupling of the HPW and SPP forms an antisymmetric ($TM_a$) and a symmetric supermode ($TM_s$) similar to a thin metal film embedded in a homogeneous dielectric bulk [6]. The $TM_a$ supermode corresponds to in-phase coupling of the HPW and SPP modes, resulting in overlap with the metal leading to significant propagation losses. On the opposite, the out-of-phase coupling of the $TM_s$ supermode minimizes overlap as a result of destructive interference. By simply tuning $t_{\varepsilon 4}$, $TM_s$ can be engineered to support long-range propagation, with modal loss that is at least an order of magnitude lower than either SPP and HPW. In this 1D analysis, the optimal $t_{\varepsilon 4}$ thickness is 148 nm for a slab mode extending to infinity in the horizontal direction.

The same loss reduction mechanism can be employed when dealing with 2D CHPW structures [5]. The effective index and propagation loss of the $TM_s$ supermode are plotted in Fig. 3 as function of the width and wavelength for a CHPW structure with optimized $t_{\varepsilon 4}$ of 185 nm. This thickness is determined based on loss optimization analysis for a minimum realizable width of 200 nm due to limitations in our fabrication processes. From the dispersion plot, it is observed that the $TM_s$ supermode of a 200 nm wide CHPW can operate up to a wavelength of $1.8\mu m$, after which the optical mode becomes leaky as the mode index drops below the substrate index.

In Fig. 3, it is observed that the propagation loss of the $TM_s$ supermode is highly tunable as a function of width, from 0.02 dB/$\mu$m at 200 nm to 1.02 dB/$\mu$m at 620 nm. This is due to the combined effects of field symmetry breaking and modal evolution asymmetry:

1. The field profiles for the $E_x$, $D_y$ and $E_z$ components are shown in Fig. 4. For $E_x$ and $E_z$, only fields inside the

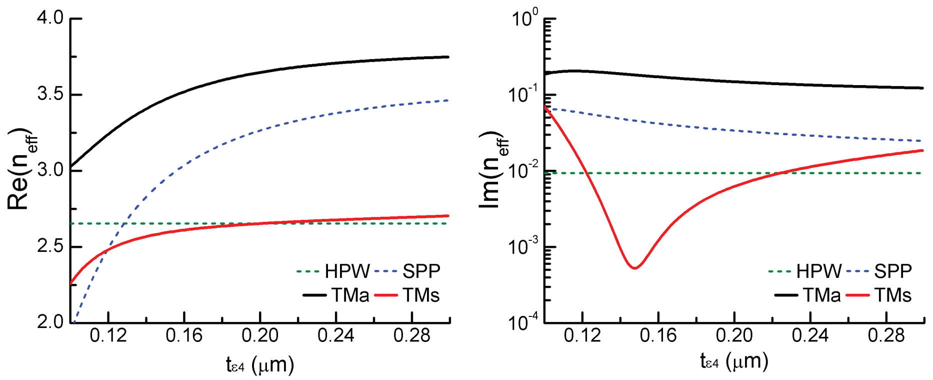


FIG. 2: Propagation constant and extinction coefficient of the decoupled HPW and SPP modes, as well as the supermodes of the CHPW in 1D.

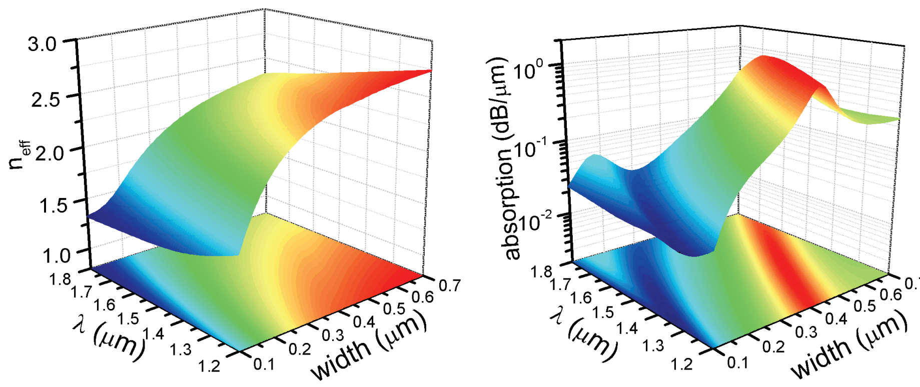


FIG. 3: Effective index and propagation loss of the CHPW symmetric supermode ($TM_s$) in 2D as function of width and wavelength. Results are calculated via 2D finite element method simulations using commercial Lumerical Mode Solutions software. Metallic boundary conditions are utilized to terminate the $2\mu$m x $2\mu$m computational domain. Grid size of 2.5 nm is used.

metal are shown. The loss contributions from $E_x$ and $E_z$ are dependent on the location of zero field-crossing. At wider widths, the overlap of $E_z$ with the metal is stronger as the position for zero-crossing does not extend to the edges as in the narrow case. On the other hand, for $E_x$ at 200 nm, a deformed quadrupole field distribution is formed from fields extending inwards from the metal corners, thus expanding the zero-crossing and reducing field overlap in two axes. As width increases, $E_x$ becomes a dipole instead and the horizontal zero-crossing is entirely shifted out of the metal, thus maximizing $E_x$ overlap.

2. The modal evolution asymmetry in the CHPW is evident in the $D_y$ profile. The higher effective index of the SPP side allows it to start supporting higher order modes at much reduced widths than the HPW side. As a result of the evolution asymmetry, the HPW can couple to higher order SPP modes to form hybridized supermodes, which increases the field overlap with the metal. In the 620 nm case, $TM_{s0}$ hybridizes with $TM_{a2}$ as their effective indices cross, but propagation loss drops again at wider dimensions as the contrast becomes larger until the next hybridization point is reached.

Note that the tunability observed here stems from the asymmetry of the CHPW and is not observed for coupled mode plasmonic waveguides that are symmetrical [4]. This enables devices that require long-range propagation and strong absorption to be fabricated simultaneously.

Because of the non-Lorentzian plasmonic field distribution, the definition used for determining the area of plasmonic modes should be chosen based on device application [7]. Since CHPW are utilized for designing active components,

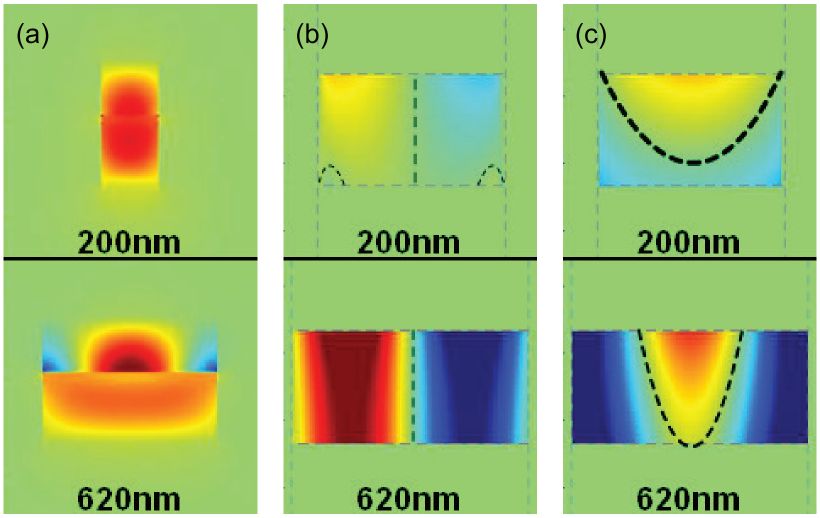


FIG. 4: (a) $D_y$, (b) $E_x$, and (c) $E_z$ profiles for the symmetric supermode at 200nm and 620 nm. For $E_x$ and $E_z$, only fields within the metal layer are shown to highlight the evolution of mode asymmetry. Dashed black line indicates where $E_x$ and $E_z$ cross zero.

strong field confinement within localized regions is important, as it leads to stronger LMI and hence shorter device length and higher energy efficiency. There, a phenomenological rather than a statistical measure of field confinement is more suitable and the effective mode area of the $TM_s$ supermode ($A$) can be defined as the ratio between the total mode energy density per unit length and the peak energy density [7]:

$$A = \frac{1}{\max\{W(\mathbf{r})\}} \int_{A_\infty} W(\mathbf{r})\,\mathrm{d}A \tag{1a}$$

$$W(\mathbf{r}) = \frac{1}{2}\mathrm{Re}\left\{\frac{\mathrm{d}[\omega\varepsilon(\mathbf{r})]}{\mathrm{d}\omega}\right\}\left|\mathbf{E}(\mathbf{r})\right|^2 + \frac{1}{2}\mu_0\left|\mathbf{H}(\mathbf{r})\right|^2 \tag{1b}$$

where $W(\mathbf{r})$ is the mode energy density. From Fig. 5, it is observed that $A$ remains relatively constant near the regime where loss is minimized. This is because the majority of the field is localized within the low-index $SiO_2$ layer and thus not sensitive to changes in $t_{\epsilon 4}$ [5]. Specifically, $A$ of 0.002 $\mu m^2$ is achieved at $t_{\epsilon 4}$=185 nm, which only changes by 5 % even with 10 % deviation in $t_{\epsilon 4}$.

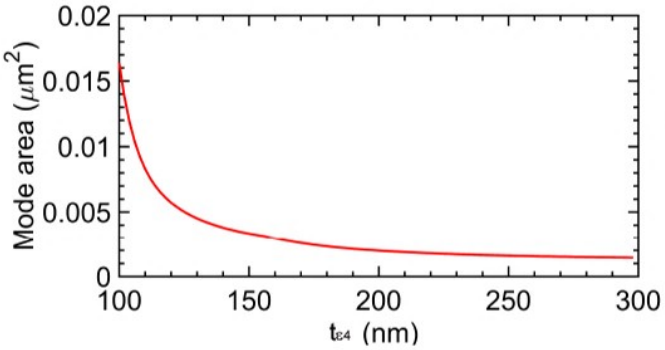


FIG. 5: Area of the $TM_s$ supermode as a function of top Si layer thickness ($t_{\epsilon 4}$).

Overall, CHPW is a robust waveguide platform that can effectively alleviate the design trade-off between mode area and propagation loss. While the loss of the CHPW is still significantly higher than that of a typical Si nanowire, it offers 55x and 6x improvement in terms of mode area and peak energy density respectively. The stronger confinement together with field enhancement can allow it to better induce non-linear effect compared to Si photonic counterparts.

| | Core cross-section [$nm^2$] | Loss [dB/$\mu$m] | Mode Area [$\mu m^2$] | Peak energy density [$J/m^3$] |
|---|---|---|---|---|
| Si nanowire (TM) | 450x220 | $0.06\times10^{-3}$ | 0.11 | $2\times10^{-11}$ |
| CHPW | 200x435 | 0.02 | 0.002 | $1.2\times10^{-10}$ |

TABLE I: Comparison between Si nanowire and CHPW

## S2 CHPW Modulator utilizing epsilon-near-zero effect

The CHPW modulator structure is schematically shown in Fig. 6(a). It has the same material layers and thicknesses as the passive CHPW components, except with an additional 10 nm ITO layer. ITO has relatively high carrier mobility around 50 $cm^2/V/s$ [8], which eliminates carrier-related device speed limitation. Concurrently, the carrier density can still be low enough such that the real part of ITO's permittivity is smaller compared to typical metals and dielectrics. This provides strong field enhancement across the ITO layer once it is placed inside a plasmonic structure with a neighboring high-index Si layer, as implied by the continuity of the displacement field.

The modulator is designed such that the loss of the $TM_s$ supermode is minimized when the bias is zero. Here, the as-deposited carrier density ($n_{den}$) of ITO is assumed to be $1 \times 10^{19} cm^{-3}$, which is required for ITO to undergo Mott transition to a metallic, degenerate-electron state [8]. As described in the main text, by changing the thickness of the top Si layer, the field overlap within the metal layer can be minimized via destructive interference. Note that the optimal thickness for the top Si is 190 nm for this modulator configuration and the ON-state loss is only 0.025 $dB/\mu m$. Therefore, the ITO layer can also be incorporated into CHPW filters and photodetectors with no change required to layer thicknesses and will have minimal performance impact.

Once a bias is applied across the Al-$SiO_2$-ITO capacitor, an electron accumulation layer is formed at the ITO-$SiO_2$ interface. A change in carrier density changes ITO's permittivity, which in turn modulates the intensity of the propagating $TM_s$ supermode (Fig. 6(b)). Specifically, for the CHPW, the field intensity and power absorbed per-unit-area are proportional to the permittivity of the ITO layer [9]. As observed in Fig. 6(c), when the local permittivity of ITO reaches a minimum of 0.57 at $6.7 \times 10^{20} cm^{-3}$, electromagnetic energy is drawn away from the high-index Si core and the $SiO_2$ layer, instead focused almost entirely within the ITO accumulation region. Due to proximity to the metal layer as well as the material absorption of ITO, the $TM_s$ mode becomes highly absorptive with modal loss >1 dB/$\mu m$.

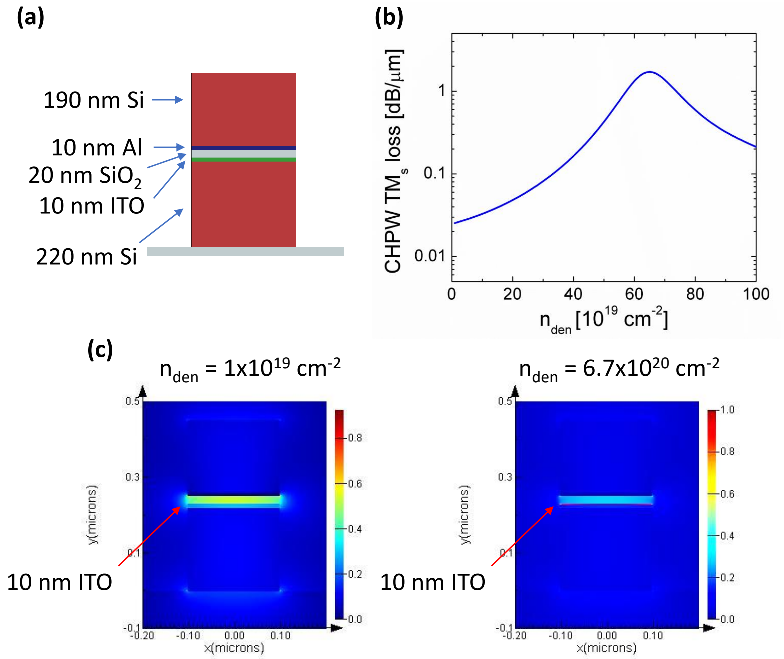


FIG. 6: (a) Schematic of the CHPW modulator. (b) Loss of the $TM_s$ supermode as a function of the carrier density inside the ITO accumulation layer. Note that an uniform accumulation layer model (1 nm) is employed as commonly used in the literature [10, 11]. (c) Simulated field distribution of the $TM_s$ supermode supported by the waveguide at $\lambda = 1550$ nm. The waveguide width is 200 nm with layers of the following thicknesses: $t_{Si,bottom} = 220$ nm, $t_{Si,top} = 190$ nm, $t_{SiO_2} = 20$ nm, $t_{ITO} = 10$ nm, $t_{Al} = 10$ nm, and $t_{SiO_{2,substrate}} = 2$ $\mu$m. Results are calculated via 2D finite element method simulations using commercial Lumerical Mode Solutions software. Metallic boundary conditions are utilized to terminate the 2 $\times$2 $\mu m^2$ computational domain. Grid size of 0.1 nm and 2.5 nm are used to mesh the accumulation layer and the rest of the waveguide structure respectively.

## S3 CHPW-Si nanowire coupler

As stated in the main text, practical chip-level optical links will require the integration of plasmonics with conventional Si photonics. To this end, efficient coupling between CHPWs and Si nanowires is mandatory (Fig 7(a)). The energy coupling between two dissimilar waveguiding systems is limited by the differences in their momentum and spatial modal distribution. However, by simply tuning the width of the Si nanowire, it is found that both mismatches can be minimized. Specifically, from Fig. 7(b), it is observed that phase match can be established at $\lambda$=1550 nm between the $TM_s$ supermode of a 200 nm CHPW and the $TM_0$ mode of a 980 nm Si nanowire. On the other hand, strong modal overlap of 77 % is achievable if the width of the Si nanowire is narrowed down to 720 nm (Fig. 7(c)). Using the Lumerical Eigenmode Expansion Solver, coupling efficiency up to 71 % can be achieved by choosing an intermediate Si nanowire width of 750 nm (Fig. 7(d)). Note that the coupler is dominated by radiation loss and the excitation of a leaky CHPW mode. Both back reflection and the excitation of $\mathrm{TM_a}$ supermode are negligible.

Using 3D FDTD simulations, the coupling efficiency into the CHPW $TM_s$ supermode is calculated to be 69% at $\lambda = 1550$ nm (Fig 8(a)). The strong coupling is sustained between $\lambda = 1450$-1650 nm and similar efficiency is observed for the reverse junction where the $TM_s$ supermode is coupled back into the Si nanowire $TM_0$ mode. Thus, dense integration between Si photonics and CHPW components is possible as efficient and broadband power transfer can occur without additional mode conversion structures. Looking at the field intensity plots in Fig. 8(b)-(d), it can be observed that a coupler length of $\sim 1\mu$m is sufficient for the electromagnetic field to stabilize after coupling from a Si nanowire into a CHPW. Due to the modal mismatch at the waveguide interface, the back reflection is calculated to be $\sim$3.3%, which results in the standing wave pattern shown in Fig. 8(b)-(d).

Note that experimental coupling efficiency was extracted to be 77 % based on cut-back measurement, which is slightly higher than the simulated value. This is attributed to better Si-CHPW modal overlap as a result of an additional 5 nm of $SiO_2$ etch-stop layer that was deposited onto the Si nanowires during fabrication.

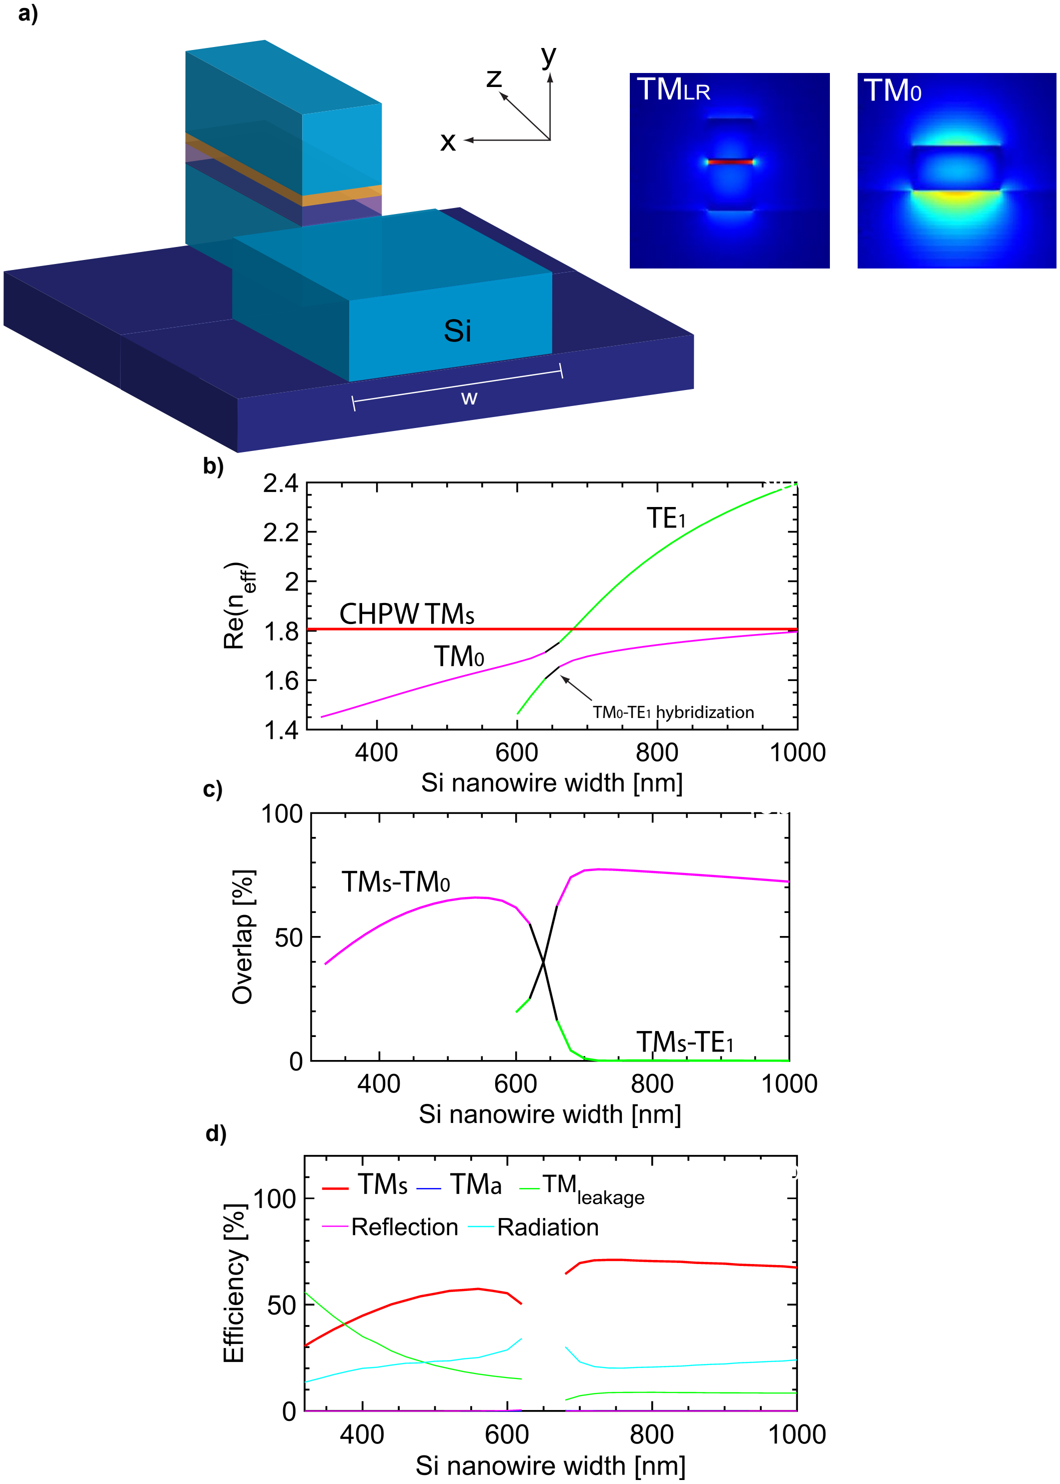


FIG. 7: **(a)** Schematic of the Si nanowire-CHPW end-fire coupler. The field profiles of the $TM_0$ mode supported by a 750 nm-wide Si nanowire and the $TM_s$ supermode supported by a 200 nm-wide CHPW are also displayed ($E_y$ is plotted). **(b)** Effective mode index of the CHPW and Si nanowire modes, calculated using Lumerical Finite Difference Eigenmode Solver at $\lambda$=1550 nm. Note that due the index difference between the air cladding and the $SiO_2$ substrate, hybridization and hence mode conversion between the $TM_0$ and $TE_1$ Si nanowire modes can occur. **(c)** Spatial modal overlap between the CHPW and Si nanowire modes. **(d)** Coupling efficiency and loss mechanisms of the Si waveguide-CHPW coupler, calculated using Lumerical Eigenmode Expansion Solver.

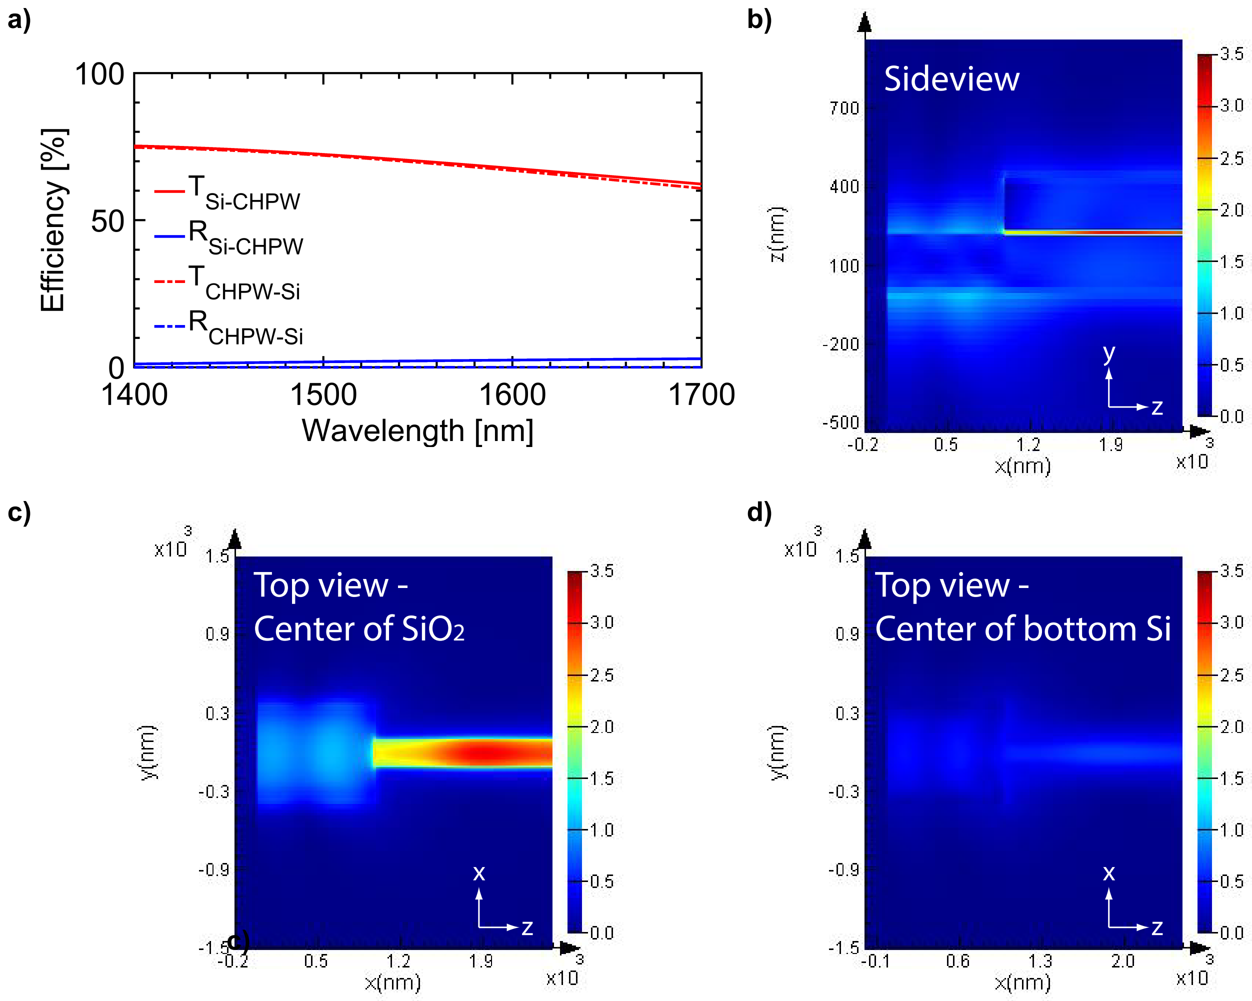


FIG. 8: **(a)** Coupling efficiency and back reflection between the $TM_0$ mode of a 750 nm Si nanowire and the $TM_s$ supermode of a 200$nm$ CHPW. **(b)-(d)** Electric field intensity patterns inside the coupler from different viewing angles as well as in different waveguide layers, obtained via 3D FDTD simulations.

## S4 CHPW Micro-ring Characteristics

The fundamental building block for the micro-ring resonator is a waveguide bend, with performance governed by radiation and propagation losses. Figure 9(a) shows the loss values for a 90 degree CHPW bend calculated using Lumerical eigenmode expansion solver. It is observed that radiation loss increases exponentially with decreasing radius ($R$). This is due to a decrease of the incident angle to a level below the critical angle required for TIR. On the other hand, propagation loss increases with increasing R due to a longer optical length. Accounting for the trade-off between the two loss mechanisms, the optimal R is determined to be 2-2.5 $\mu$m and the lowest bending loss is $\sim$0.15dB. Note that we have only manipulated the thickness of the top Si layer to optimize the waveguide propagation loss in this work. It is expected that the optimization of other waveguide layers can further reduce the propagation loss and improve the Q-factor.

The calculated loaded Q-factor ($Q$) for a 200 nm wide CHPW micro-ring resonator with $R$=2.05 $\mu$m is shown in Fig. 9(b). The resonance wavelength is 1538 nm at 20°C. By reducing the coupling coefficient ($\kappa$), the ring can operate in the under-coupled regime. As such, $Q$ can approach the intrinsic Q-factor of $\sim$3400 asymptotically, albeit a trade-off in the extinction ratio. As temperature increases, the resonant wavelength red-shifts but there is little degradation in $Q$ unless $\kappa$ is changed significantly. From Fig. 9(c), it is further observed that the coupling length between the Si bus and the CHPW ring waveguide is also not strongly influenced by temperature. The coupling length exhibits slight decrease with increasing temperature, corresponding to an increase in $\kappa$ and thus a decrease in $Q$, which matches with the trend observed in our experimental result (Figure 10(c)).

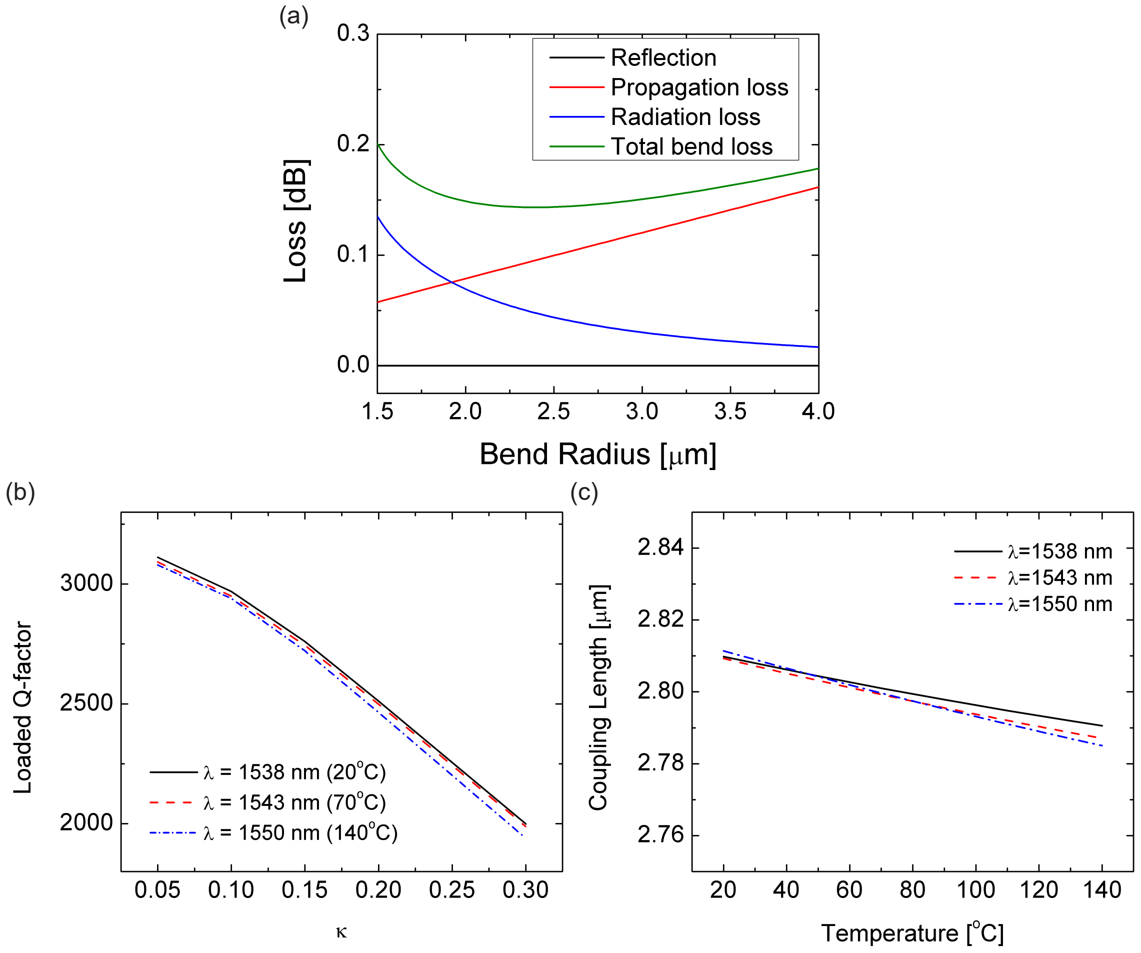


FIG. 9: (a) Loss mechanisms inside a CHPW bend. (b) Loaded quality factor at different chip temperatures and resonant wavelengths as a function of coupling coefficient ($\kappa$) for a CHPW micro-ring with 2.05 $\mu$m radius. (c) Coupling length between the Si bus and CHPW ring waveguide for different chip temperatures and resonant wavelengths.

### S5 CHPW Micro-ring Characterization

To demonstrate the applicability of the CHPW platform for filtering and optical emission, all-pass Si-to-CHPW microring resonators have been fabricated and characterized. To reduce measurement noise, light from the tunable laser is chopped at a randomly-selected frequency of 377 Hz and the ring output is measured via an locked-in amplifier. The micro-rings have been tested at varying temperatures to investigate the sensitivity of the resonance conditions. Substrate temperature is fine-tuned using a custom copper stage with thermoelectric coolers, where temperature is adjusted using a Keithley 2510-AT Autotuning TEC source meter through the electrical feedback from a 10k thermistor. The measured ring spectra are shown in Fig. 10(a), where fringes with smaller free spectral range and extinction ratio are also observed due to cavities formed by the input and output Si nanowires. For a CHPW resonator with radius of 2.5 $\mu$m and gap width of 215 nm, the resonance undergoes red-shift at $\sim$80pm/C. Due to limitation in the power output of the thermoelectric cooler source meter, the pelltiers need to operate in a voltage-limited regime and thus stage temperature constantly fluctuates by up to 0.2$\circ$C during measurement. This introduces fluctuation to the measurement result. Additional uncertainly also exists as the set-up is manually realigned to obtain maximum waveguide power output at each temperature. Nonetheless, the loaded Q-factor and ER are maintained around 3000 and 10 dB respectively (Fig. 10(b) to (d)).

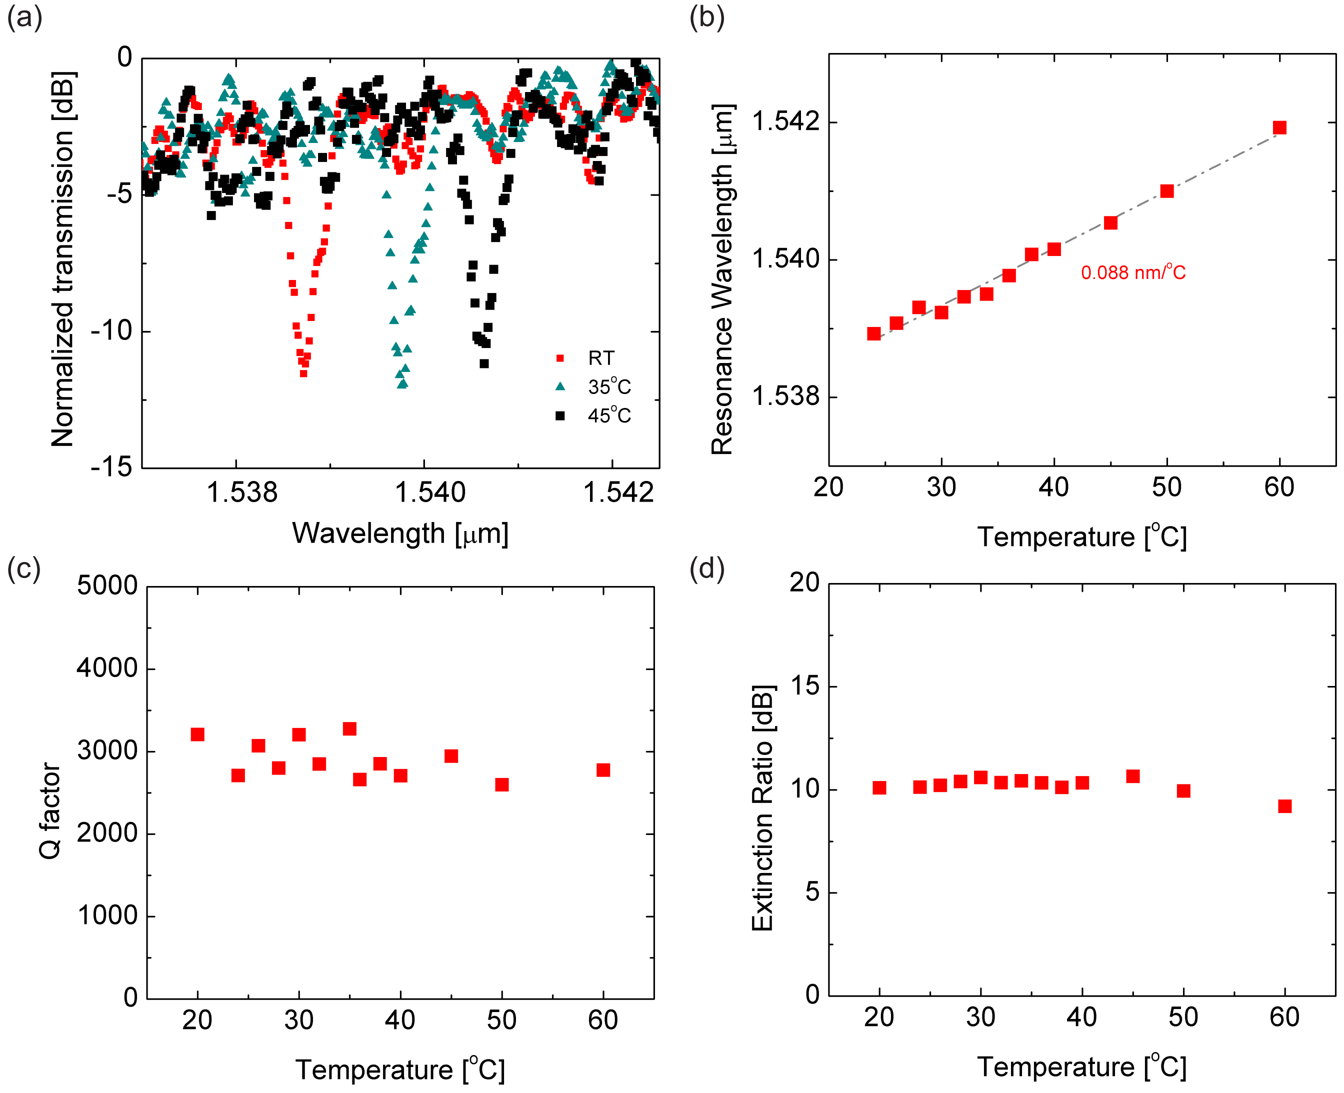


FIG. 10: (a) Transmission spectra at different temperatures for CHPW ring resonator. (b) Resonant wavelength of the CHPW ring at different substrate temperatures (c) Loaded Q-factor of the CHPW ring at different substrate temperatures (d) Extinction ratio of the CHPW ring at different substrate temperatures.

### S6 RC Bandwidth of CHPW Photodetectors

To estimate the RC bandwidth, the parasitic capacitances of the CHPW photodetectors have been measured using a HP4280 1MHz C Meter (Fig. 11). The total device capacitance, which includes contributions from the photodetector, the fingers, contact pads, and substrate, increases from 8 to 12 fF as photodetector length is increased from 5 to 20 $\mu$m. Neglecting resistance from the Al contact pads, the upper limit of the RC bandwidth for a 5 $\mu$m device is calculated to be 398 GHz assuming 50$\Omega$ load. Note that speed of the current device may also be limited by carrier transit time, which is governed by the saturation drift velocity of $\alpha$-Si [12]. in that case, future device generations can alleviate this limitation through controlled doping profiles as well as reducing the $\alpha$-Si layer thickness to reduce transit time.

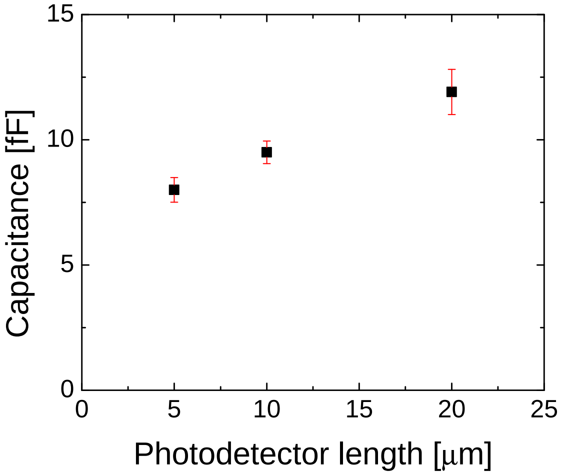


FIG. 11: Measured capacitance of the fabricated CHPW photodetectors at 4 V.

### S7 Comparison of Experimental Plasmonic Photodetectors based on internal photoemission (IPE)

A comparison between experimental demonstrations of IPE-based plasmonic photodetectors is displayed in Table II. Despite the use of $\alpha$-Si, the CHPW photodetector showcases a record sensitivity of -54 dBm at 2 V and can maintain a <-40 dBm sensitivity across large voltage, bandwidth, and temperature conditions. Note that although the slot waveguide-based design has outperformed the CHPW in terms of responsivity ($R$), it uses a narrower Si region. Both designs have $R$ in the range of few 10s of mA/W if the Si dimension is 200 nm.

The $R$ of CHPW photodetector is roughly one order of magnitude lower than the values measured for state-of-the-art SiGe devices [13]. This can be improved through the use of a narrower $\alpha$-Si region to reduce the transport loss. Moreover, although the dark current level of the CHPW photodetector is already significantly lower compared to its plasmonic counterparts, it can be further suppressed by using metals with higher barrier at the non-emitting Schottky junction [14].

| | Device Junction | Length ($\mu$m) | $R$ at 1550 nm ($mA/W$) | $I_d$ (nA) | $S_{min}$ ($dBm$) | Speed (GHz) |
|---|---|---|---|---|---|---|
| Strip waveguide [15] | Al-$c$Si | 35 | 0.8 | 6000 ($0.1V$) | 8 | — |
| Strip waveguide [16] | Au-$c$Si | $40-60$ | 1 | — | — | — |
| Silicide on SOI [17] | $NiSi_2$-$c$Si | 23.4 | 4.6 | 3 ($1V$) | $-30$ | 2 |
| MSM [18] | Cu-$c$Si | — | $1.5-4.5$ | 1.8-2.2 ($5-21V$) | $-29$ | — 1 |
| Slot waveguide [14] | Au-$c$Si-Ti | $4-20$ | $14-126$ | 300-10000 ($1-3V$) | $-16$ | 40 |
| CHPW [19] | Al-$\alpha$Si | $5-20$ | $0.5-5$ | 0.05-100 ($6-15V$) | $-35$ | 2.5* |
| CHPW | Al-$\alpha$Si | $5-20$ | $1-80$ | 0.05-100 ($2-10V$) | $-54$ | 26* |

* limited by instrumentation

TABLE II: Comparison of experimentally demonstrated, travelling-wave plasmonic photodetectors based on IPE

### S8 Characterization of CHPW modulators

The transmission of 10 $\mu$m CHPW modulators under forward-bias is shown in Fig. 12(a). The maximum voltage is kept below 26 V to prevent oxide breakdown and the results have been normalized with respect to optical transmission at zero bias. It is observed that optical transmission decreases slowly with voltage up to 20 V, after which a sharp increase in optical absorption occurs and transmission is reduced to -10 dB at 25 V. This corresponds to strong extinction ratio (ER) of 1 dB/$\mu$m, one of the highest measured to-date. For comparison, the behavior of the same modulator under reverse-bias as well as a modulator without an ITO layer are also measured. As no modulation can be observed under both scenarios, the measured modulation response can indeed be attributed to field-induced carrier-accumulation instead of drift in the set-up, thermal-optic effect at high bias voltage, or electro-optic effect in materials other than ITO. Moreover, modulation depth varies with device length and the normalized transmission for a 15 $\mu$m modulator can reach -12 dB at 26 V (Fig. 12(b)).

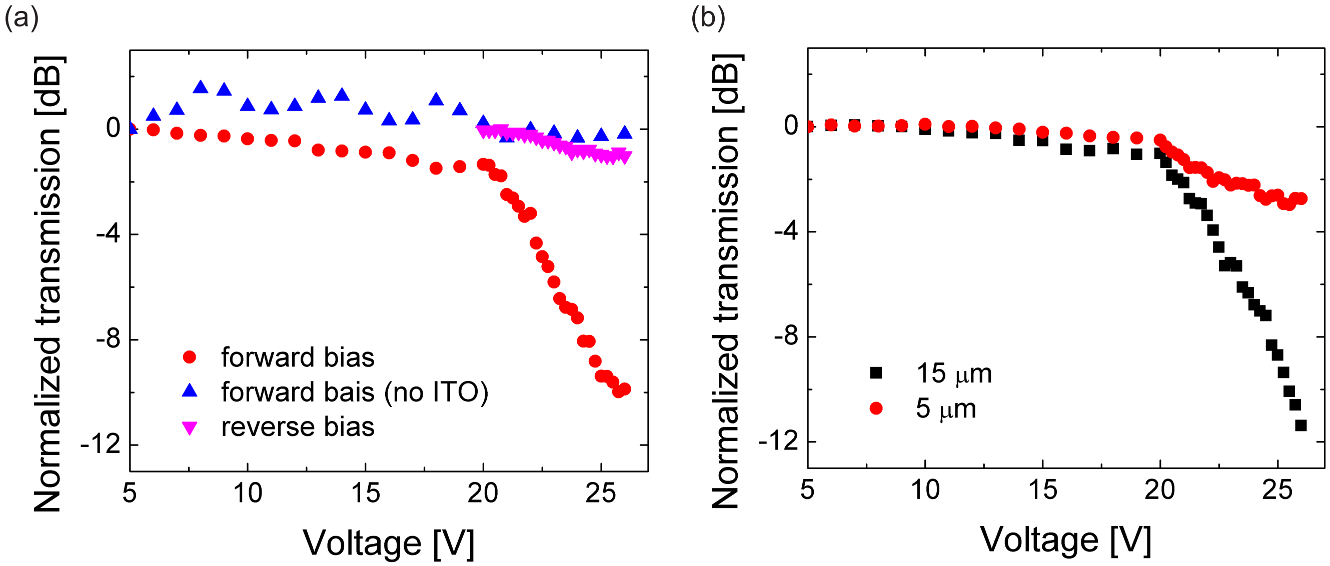


FIG. 12: **(a)** Normalized transmission of 10 $\mu$m CHPW modulator as a function of bias. The behavior of a modulator without an ITO layer is also displayed. **(b)** Normalized transmission of 5 and 15 $\mu$m CHPW modulators.

The performance of the CHPW modulator is characterized over broad temperature and wavelength conditions. The difference in modulator ER at room and elevated temperatures is shown in Fig. 13 for a 10 $\mu$m CHPW modulator. Due to limitation in the power output of the TEC source meter, the pelltiers need to operate in a voltage-limited regime and thus stage temperature can fluctuate by up to 0.2 °C. In spite of the noise caused by tool fluctuation, modulator ER does not degrade and in fact increases with temperature. Specifically, a 0.75 dB increase in ER is observed at 100 °C and V = 25V. This improvement may be attributed to the temperature dependence of ITO's resistivity and requires future study.

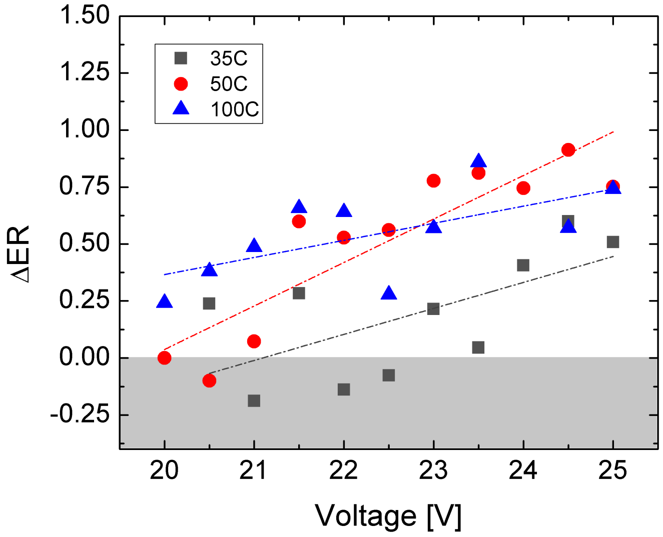


FIG. 13: Change in the extinction ratio of 10 $\mu$m CHPW modulator at elevated temperatures. The results have been normalized with respect to device response at room temperature.

## S9 RC Bandwidth of CHPW Modulators

The speed of the CHPW modulator is governed by two factors: (1) the formation/deformation time of the accumulation layer inside ITO and (2) the capacitive RC-delay time. Electron accumulation is a fast process based on majority carrier dynamics and the formation time can be calculated via $\tau = t_{ITO}/\nu_{drift}$, where $t_{ITO}$ = 10 nm and $\nu_{drift}$ are the thickness and carrier drift velocity of ITO respectively. More specifically, $\nu_{drift}$ can be estimated via $\nu_{drift} = \mu E$, where $\mu$ is ITO's mobility and $E$ is the applied electric field which is proportional to the gate voltage divided by the oxide thickness ($t_{SiO_2}$= 20 nm). Using $\mu$=33 $cm^2/Vs$ as obtained through Hall measurement, the resulting speed exceeds 300 THz. Similarly, the electron scattering rate of ITO is $\sim$ 290 THz and therefore the modulator speed is also not limited by the carrier transient response when the gate bias is turned off [20]. Hence, similar to other MOS-based modulators, the speed of the CHPW modulator is dictated by the RC constant [21]. With parasitic capacitance of 5 fF, the upper limit of the bandwidth for the 10 $\mu$m modulator is calculated to be 636 GHz assuming a 50 $\Omega$ load resistance. Since the response of light to the plasma dispersion effect is much faster than the RC limit, any delay from the decay of strong local fields can be neglected. Hence, the electrical modulation speed of 636 GHz directly translates to the optical domain.

## S10 Comparison of Experimental ITO-based Plasmonic Modulators

A comparison of the CHPW modulator against other experimentally realized ITO-based modulators is shown in Table III. The ER of the CHPW modulator can be as high as that of a HPW modulator. Concurrently, although the ITO carrier density being an order of magnitude higher, the CHPW modulator still has the lowest reported insertion loss (IL) and the highest optical figure-of-merit (ER/IL) to-date. Although currently limited by the bandwidth of the testing instruments, the CHPW's experimental modulation speed of 26 GHz is also the highest reported to-date. Thus, CHPW's potential for implementing optical modulators with compact footprint, high ER per device length, low IL, as well as broadband and high-speed operation is clearly demonstrated.

| Waveguide | Gate oxide | $n_{den}$ of ITO ($10^{19} cm^{-3}$) | IL ($dB/\mu m$) | ER ($dB/\mu m$) | ER/IL | Bandwidth (GHz) |
|---|---|---|---|---|---|---|
| CHPW | $SiO_2$ (20 nm) | 20 | 0.095 | 1 | 9.09 | 26 |
| HPW[9] | $SiO_2$ (20 nm) | 1.1 | 0.14 | 1 | 7.14 | - |
| MIM[11] | $Al_2O_3$ (5 nm) | 1.6 | 0.45 | 2.7 | 6 | - |
| Si[22] | $HfO_2$ (10 nm) | 4.9 | 2.5 | 1.6 | 0.64 | 1.25 |

TABLE III: Comparison of experimentally demonstrated ITO-based modulators.

## S11 Simulated Eye Diagrams

To investigate the digital time domain performance of CHPW devices, we have generated simulated eye diagrams that are based on our experimental results. Specifically, compact models for CHPW modulator, CHPW photodetector, and Si-CHPW couplers have been implemented using the experimentally measured responses, bandwidths, and parasitics. As shown in Fig. 14, photonic links are then constructed and simulated by using a combination of the CHPW compact models and the validated device models from the process design kit provided by the American Institute for Manufacturing Integrated Photonics (AIM photonics) [23]. The optical input is coupled into the chip via grating couplers and the electrical output is amplified through transimpedance amplifier (TIA). The link architectures are representative of how Si photonic modulators/detectors are tested in an integrated on-chip setting. The device properties used in the circuit simulations have been tabulated in Table IV. In our simulations, the CHPW modulator operates at 25V and has a RC-limited bandwidth of 31 GHz, calculated using the experimental contact and series resistances (1 kΩ) and capacitance (3 fF). The CHPW photodetector operates at 10V and is assumed to have a transient-limited bandwidth of 50 GHz, calculated using a saturation drift velocity of $10^6$ cm/s for the 200 nm top $\alpha$-Si layer [12]. Note that the thickness of the $\alpha$-Si is chosen to match with that of the ring in order to demonstrate the versatility of the structure. Thickness reduction in future fabrication runs will enable the CHPW photodetectors to become RC-limited.

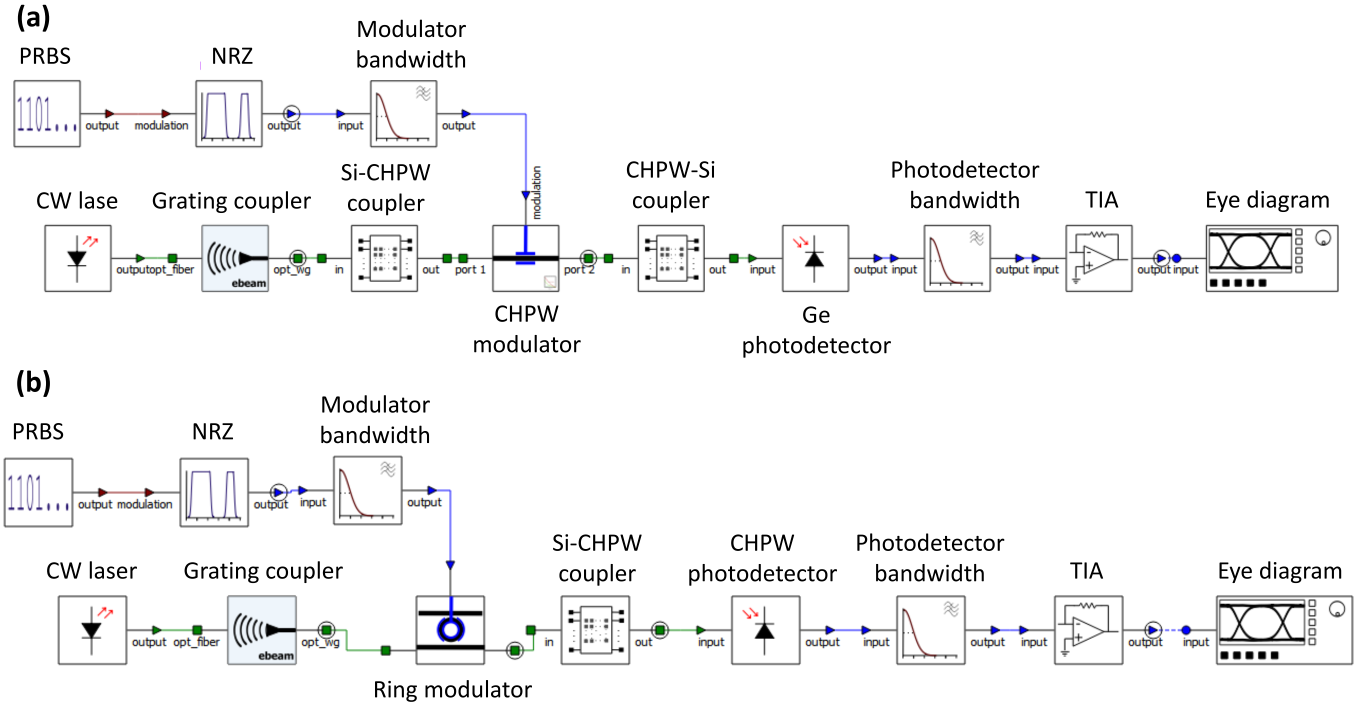


FIG. 14: Schematic views in Lumerical Interconnect for the link architectures for (a) CHPW modulator characterization and (b) CHPW photodetector characterization.

Figures 15(a) to (c) display the simulated CHPW modulator eye diagram for 10 Gbps, 25 Gbps, and 50 Gbps respectively. Open eye patterns are observed, corresponding to minimal signal distortion. Similarly, the link containing the CHPW photodetector is also functional up to 50 Gbps (Figures 15(d) to (f)), albeit larger eye closures due to smaller Si ring modulator bandwidth and higher photodetector dark current compared to the link for testing CHPW modulator. Note that the simulations described here do not accounted for the total noise of the system. Parasitics such as noises from the optical source and its amplifiers, loss and bandwidth limitations of the RF cables and bias tee, or RF mismatches at the contact region will impose additional limitations on the opening of the eye pattern.

| Device | Property | Value |
|---|---|---|
| Laser | Power | 3 mW |
| Grating coupler | Loss | 1.5 dB |
| Si ring modulator | Insertion loss | 1.2 dB |
| Si ring modulator | Extinction ratio | 4.83 dB |
| Si ring modulator | Bandwidth | 17 GHz |
| Ge photodetector | Responsivity | 1 A/W |
| Ge photodetector | Dark current | 50 nA |
| Transimpedance amplifier | Transimpedance | 1 kΩ |
| Transimpedance amplifier | Equivalent input noise | 2.4 $\mu$A |

TABLE IV: Properties of devices from the AIM Photonics PDK.

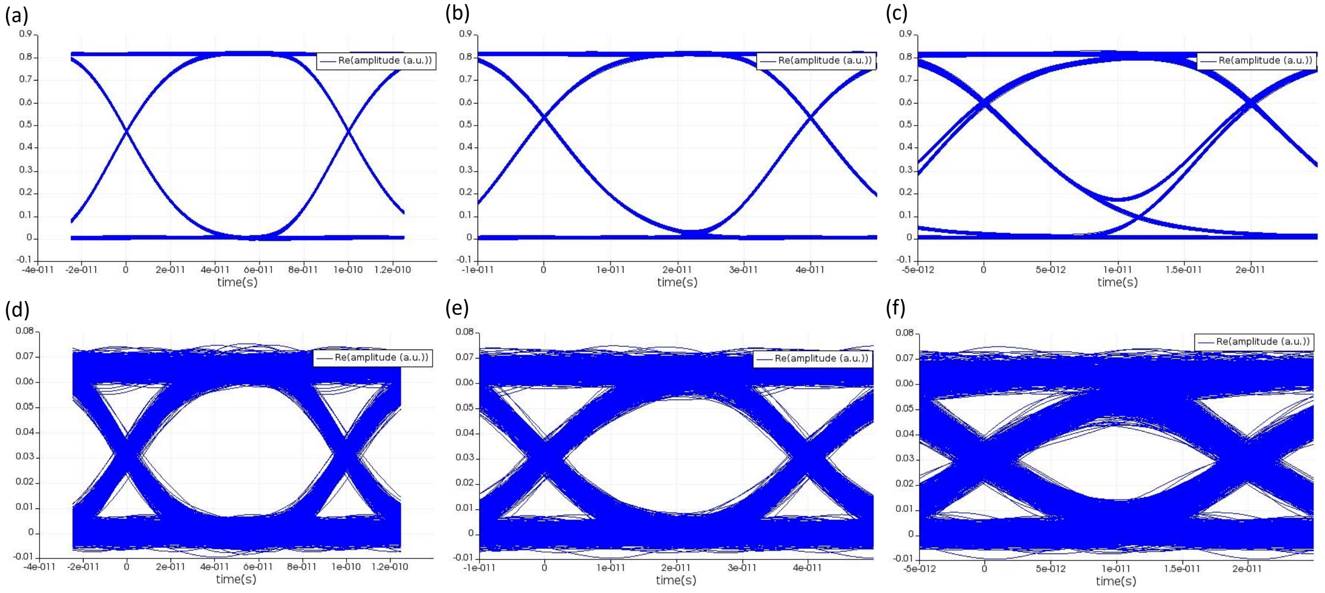


FIG. 15: (a)-(c) Simulated eye diagrams for 10 $\mu$m long CHPW modulator at 10, 25, and 50 Gbps. (d)-(f) Simulated eye diagrams for 15 $\mu$m long CHPW photodetector at 10, 25, and 50 Gbps.


[1] Bozhevolnyi, S. I. Plasmonic Nanoguides and Circuits. (*CRC Press Book*, (2009)).

[2] Bian, Y., Zheng, Z., Zhao, X., Zhu, J. & Zhou, T. Symmetric hybrid surface plasmon polariton waveguides for 3d photonic integration. *Optics Express* **17,** 21320-21325 (2009).

[3] Chen, L., Li, X., Wang, G., Li, W., Chen, S., Xiao, L., & Gao, D. A silicon-based 3-d hybrid long-range plasmonic waveguide for nanophotonic integration. *Journal of Lightwave Technology* **28,** 163-168 (2012).

[4] Ma, W. & Helmy, A. S. Asymmetric long-range hybrid-plasmonic modes in asymmetric nanometer-scale structures. *Journal of the Optical Society of America B* **31,** 1723-1729 (2014).

[5] Su, Y., Chang, P, Lin, C., & Helmy, A. S. Record Purcell factors in ultracompact hybrid plasmonic ring resonators. *Science Advances* **5,** eaav1790 (2019).

[6] Berini, P. Plasmon-polariton waves guided by thin lossy metal films of finite width: Bound modes of asymmetric structures. *Physical Review B* **63,** 125417 (2001).

[7] Oulton, R. F., Bartal, G., Pile, D. F. P., & Zhang, X. Confinement and propagation characteristics of subwavelength plasmonic modes. *New Journal of Physics* **10,** 105018 (2008).

[8] P. P., Edwards, Porch, A. Jones, M. O. Morgan, D. V. & Perks, R. M. Basic materials physics of transparent conducting oxides. *Dalton Transactions* **19,** 2995-3002 (2004).
[9] Sorger, V. J., Lanzillotti-Kimura, N. D., Ma, R., & Zhang, X. Ultra-compact silicon nanophotonic modulator with broadband response. *Nanophotonics* **1,** 17-22 (2012).
[10] Vasudev, A. P., Kang, J., Park, J., Liu, X., & Brongersma, M. L. Electro-optical modulation of a silicon waveguide with an "epsilon-near-zero" material. *Optics Express* **21,** 26387-26397 (2013).
[11] Lee, H. W., Papadakis, G., Burgos, S. P., Chander, K., Kriesch, A., Pala, R., Peschel, U., & Atwater, H. A. Nanoscale Conducting Oxide PlasMOStor. *Nano Letters* **14,** 646-6468 (2014).
[12] Maassen, J., Yelon, A., & Hamel, L. A. Simulation of picosecond domain time-of-flight experiments in aSi:H. *Journal of Non-Crystalline Solids* **353,** 4779-4782 (2007).
[13] Tseng, C.-K., Chen, W.-T., Chen, K.-H., Liu, H.-D., Kang, Y., Na, N., & Lee, M.-C. M. A self-assembled microbonded germanium/silicon heterojunction photodiode for 25 Gb/s high-speed optical interconnects. *Scientific Reports* **3,** 3225 (2013).
[14] Muehlbrandt, S. Melikyan, A., Harter, T., Kohnle, K., Muslija, A., Vincze, P., Wolf, S. Jakobs, P., Fedoryshyn, W. Freude, W., Leuthold, J., Koos, C., & Kohl, M. Silicon-plasmonic internal-photoemission detector for 40 Gbit/s data reception. *Optica* **3,** 741-747 (2016).
[15] Akbari, A., Tait, R., & Berini, P. Surface plasmon waveguide Schottky detector. *Optics Express* **18,** 8505-8514 (2010).
[16] Berini, P., Olivieri, A., & Chen, C. Thin Au surface plasmon waveguide Schottky detectors on p-Si. *Nanotechnology* **23,** 444011 (2012).
[17] Zhu, S., Yu, M., Lo, G. & Kwong, D. Near-infrared waveguide-based nickel silicide Schottky-barrier photodetector for optical communications. *Applied Physics Letters* **92,** 081103 (2008).
[18] Casalino, M., Iodice, M., Sirleto, L., Rendina, I. & Coppola, G. Asymmetric MSM sub-bandgap all-silicon photodetector with low dark current. *Optics Express* **21,** 28072-28082 (2013).
[19] Su, Y., Lin, C., Chang, P., & Helmy, A. S. Highly sensitive wavelength-scale amorphous hybrid plasmonic detectors. *Optica* **10,** 1259-1262 (2017).
[20] Michelotti, F., Dominici, L., Descrovi, E., Danz, N., & Menchini, F. Thickness dependence of surface plasmon polariton dispersion in transparent conducting oxide films at 1.55 $\mu$m. *Optics Letters* **34,** 839-841 (2009).
[21] Liu, A., Jones, R., Liao, L., Samara-Rubio, D., Rubin, D., Cohen, O., Nicolaescu, R., & Paniccia, M. A high-speed silicon optical modulator based on a metal-oxide-semiconductor capacitor. *Nature* **427,** 615-618 (2004).
[22] Wood, M. G., Campione, S., Parameswaran, S., Luk, T. S., Wendt, J. R., Serkland, D. K., & Keeler, G. A. Gigahertz speed operation of epsilon-near-zero silicon photonic modulators. *Optica* **5,** 233-236 (2018).
[23] Process Design Kit (PDK). http://www.aimphotonics.com/pdk (accessed 2020-03-06).
